# Supplementary material for: HOMURA: Taming the Sand-Glass for Time-Constrained LLM Translation via Reinforcement Learning
Source: arXiv:2601.10187 source file (2026-09-03)
Supplement: Supplementary file 1 [file Appendix.tex]

\section{Related Work}
\label{sec:appendix_related_works}
\subsection{Constrained Translation and Subtitling}
Media localization imposes strict spatiotemporal constraints beyond semantic fidelity \citep{karakanta-etal-2020-must}. To address these limitations, early research focused on supervised learning paradigms that integrate specialized markers to guide line length and reading speed \citep{karakanta-etal-2020-42}. An advancement was introduced by \citet{wu-etal-2023-videodubber} with \textit{VideoDubber}, which pioneered direct speech-length control by incorporating token-level duration predictions into the decoder stack. However, this approach remains constrained by its dependence on supervised training with non-isochronous datasets and heuristic duration labeling that introduces annotation noise. Building on this, \citet{chadha2025lengthawarespeechtranslation} demonstrated that even with automatically generated length tags derived from phoneme ratios, supervised training on non-isochronous speech-translation data remains a fundamental bottleneck for achieving precise isochronicity. While architectures like CLSC \citep{jorgensen-mengshoel-2025-cross} further refine this task using control tokens to manage sequence length, they remain fundamentally dependent on supervised training with task-specific compression corpora. In contrast, our work targets general-purpose Large Language Models (LLMs) via a reinforcement learning framework. This approach explicitly optimizes the trade-off between semantic preservation and temporal compliance without requiring ground-truth compression datasets.

\subsection{Hard Constraints and Lyric Translation}
The imposition of strict feasibility constraints parallels automatic lyric translation, where models must adhere to syllable counts and rhythm \citep{ou-etal-2023-songs}. Building on curriculum RL strategies for discrete constraints \citep{ren2025lyricar}, \textit{HOMURA} treats temporal duration as a hard constraint. We employ a KL-regularized objective to balance these rigid length requirements with semantic quality, ensuring the model respects the "sand-glass" temporal budget.

\subsection{Verbosity Bias in LLMs}
A major challenge for time-constrained translation is the systemic "verbosity bias" in LLMs, often exacerbated by RLHF alignment that conflates length with helpfulness \citep{saito2023verbosity, skalse2022defining, singhal2023long}. Our framework counteracts this by introducing a dynamic syllable-ratio reward. Instead of encouraging length drift, we specifically penalize verbosity, aligning the model's output with the strict density requirements of subtitling and dubbing.


\section{Statistical Significance Testing}
\label{sec_statistical_test_appendix}

We perform hypothesis testing to examine whether the improvements brought by HOMURA are statistically significant.
For a fair comparison, for each baseline we choose its best-performing configuration that (i) requires a single inference pass and (ii) satisfies the target in-bounds constraint (IB), and compare it with HOMURA under the same constraints.
Table~\ref{tab:statistical_sign_test} reports the resulting p-values.

\begin{table}[th]
    \centering
    \caption{p-values for testing HOMURA against each variant.}
    \label{tab:statistical_sign_test}
    
    \setlength{\tabcolsep}{5pt}
    \renewcommand{\arraystretch}{1.1}

    \resizebox{0.7\linewidth}{!}{%
    \begin{tabular}{l|ccc|ccc}
        \toprule
        \textbf{Model} & \multicolumn{6}{c}{\textbf{p-value of HOMURA}} \\
        \cmidrule(lr){2-7}
        & \multicolumn{3}{c|}{\textbf{Zh $\rightarrow$ En}} & \multicolumn{3}{c}{\textbf{Zh $\rightarrow$ De}} \\
        \cmidrule(lr){2-4}\cmidrule(lr){5-7}
        & \textbf{IB} & \textbf{BLEU-$\rho$} & \textbf{COMETKiwi}
        & \textbf{IB} & \textbf{BLEU-$\rho$} & \textbf{COMETKiwi} \\
        \midrule
        \textbf{HOMURA\textsubscript{Rubric}}
          & $\checkmark$ & 6.46e-03 & 8.20e-03
          & $\checkmark$ & $<\!1e\!-\!10$        & $<\!1e\!-\!10$ \\
        \textbf{HOMURA\textsubscript{Reason}}
          & $\checkmark$ & - & 6.30e-03
          & $\checkmark$ & $<\!1e\!-\!10$ & $<\!1e\!-\!10$ \\
        \bottomrule
    \end{tabular}%
    }
    \vspace{2mm}
\end{table}

Across both language pairs and evaluation metrics, HOMURA yields statistically significant improvements over its strongest single-pass, in-bounds baselines, with p-values consistently below the conventional 0.01 threshold (often far smaller, e.g., $<\!1e\!-\!10$ for Zh$\rightarrow$De). These results confirm that the observed gains are unlikely to be due to random variation. The ``--'' entry denotes a degenerate case where the two compared results are identical, yielding no measurable difference and thus no meaningful significance test.
For Zh$\rightarrow$Es, no baseline satisfies the single-pass and in-bounds constraints, and thus we do not conduct hypothesis testing.

\section{Human Evaluation}
\label{sec:appendix_human_judgment}
We additionally report human evaluation results for the Zh-to-En setting to further validate the effectiveness of our method and the appropriateness of our evaluation metrics.

\begin{table}[h]
\centering
\caption{Human evaluation results on Accuracy and Completeness under different settings. Note: IB: In Bounds, $\checkmark$ indicates within bounds, $\times$ indicates out of bounds.}
\label{tab:human_eval_acc_comp}
\setlength{\tabcolsep}{1.5pt}
\renewcommand{\arraystretch}{1.0}
\footnotesize
\resizebox{0.7\linewidth}{!}{%
\begin{tabular}{@{}p{2.25cm}lccccc@{}}
\toprule
\textbf{Setting} & \textbf{Model} & \textbf{IB} & \textbf{Accuracy} & \textbf{Completeness} & \textbf{Avg.}\\
\midrule
\multirow{4}{*}{w/o syll.} 
& Gemini-2.5-Pro   & $\times$ & 4.95 & 5.00 & 4.97\\
& Claude-4.1-Opus  & $\times$ & 4.91 & 4.98 & 4.94\\
& GPT-5            & $\times$ & 4.96 & 5.00 & 4.98\\
& DeepSeek-V3      & $\times$ & 4.97 & 5.00 & 4.99\\
\midrule
\multirow{4}{*}{w/ syll.} 
& Gemini-2.5-Pro   & $\times$ & 4.44 & 4.90 & 4.67\\
& Claude-4.1-Opus  & $\checkmark$ & 4.42 & 4.93 & 4.67\\
& GPT-5            & $\times$ & 4.42 & 4.87 & 4.65\\
& DeepSeek-V3      & $\times$ & 4.42 & 4.87 & 4.65\\
\midrule
\multirow{4}{*}{Best-of-$N$} 
& Gemini-2.5-Pro   & $\checkmark$ & 4.57 & 4.57 & 4.57\\
& Claude-4.1-Opus  & $\checkmark$ & 4.51 & 4.49 & 4.50\\
& GPT-5            & $\checkmark$ & 4.71 & 4.80 & 4.75\\
& DeepSeek-V3      & $\checkmark$ & 4.56 & 4.58 & 4.57\\
\midrule
\multirow{2}{*}{Ours} 
& HOMURA\textsubscript{Rubric} & $\checkmark$ & 4.91 & 4.83 & 4.87\\
& HOMURA\textsubscript{Reason} & $\checkmark$ & 4.85 & 4.93 & 4.89\\
\bottomrule
\end{tabular}%
}
\end{table}

Table~\ref{tab:human_eval_acc_comp} shows that (i) without syllable constraints, all frontier LLMs achieve near-ceiling Accuracy/Completeness, serving as an unconstrained upper bound; (ii) enforcing syllable budgets by prompting substantially degrades human-rated quality, especially Accuracy; and (iii) Best-of-$N$ provides limited and unstable gains. In contrast, our HOMURA variants deliver the best overall constrained performance, approaching the unconstrained ceiling, with HOMURA\textsubscript{Rubric} slightly favoring Accuracy and HOMURA\textsubscript{Reason} favoring Completeness.




\section{The Sand-Glass Benchmark Construction}
\label{sec:appendix_sand-glass_construction}

Sand-Glass is designed for \emph{time-constrained} translation, where the output must satisfy a strict temporal budget while preserving essential meaning. 
The construction emphasizes two components: 
(i) \textbf{duration-aware segmentation} to derive realistic per-segment budgets from natural speech, 
and (ii) \textbf{core event extraction} to enable a fine-grained semantic retention check under forced compression (facilitating the \textit{BT-CERR} metric defined in Sec.~\ref{sec:evaluation_metrics}).

\paragraph{Pipeline Overview.}
Starting from real-world video datasets across diverse specialized domains, we extract ASR transcripts, segment them into duration-bounded subtitle units, apply multi-stage quality filtering (including strict length constraints), and finally extract \emph{core events} (predicate--argument abstractions) to serve as a semantic backbone.

\paragraph{Construction Procedure.}
\begin{enumerate}
    \item \textbf{Data Acquisition and Segmentation.}
    We collect a large-scale corpus of real-world video transcripts covering five representative domains: \textit{Gaming}, \textit{Film \& Television}, \textit{Travel \& Tourism}, \textit{ACGN (Animation, Comics, Games and Novels)}, and \textit{General Knowledge}. Speech is transcribed via ASR and segmented based on pauses and semantic units. Each segment is assigned a temporal budget derived from its actual speech duration. 
    
    \item \textbf{Preprocessing and Packaging.}
    We strip non-speech artifacts (e.g., fillers, music markers) and package segments into sliding windows of ten to preserve contextual coherence. Outputs are enforced into a fixed JSON schema for model interaction.
    
    \item \textbf{Multi-stage Quality Filtering.}
    We apply a rigorous filtering pipeline to ensure structural and linguistic integrity. 
    \textit{Statistical Sanity:} To ensure the statistical stability of the $\rho$ metric, we exclude segments with fewer than 10 characters or extreme Characters-Per-Second (CPS) values. This prevents short-sequence outliers from inflating density results and ensures that temporal constraints necessitate meaningful semantic compression. 
    \textit{Quality Heuristics:} Samples are scored via an ensemble of signals—including perplexity, repetition, and script consistency—retaining borderline cases with lower weights to preserve a natural difficulty curve. 
    \textit{Diversity:} Following LSH-based de-duplication \cite{jha2023limit}, we perform \textit{domain-balanced quota sampling} to obtain a high-quality final corpus of \textit{1,000 golden instances}. This ensures a representative and manageable distribution of expansion challenges across the five selected domains.

    \item \textbf{Core Event Extraction.}
    Since compression increases the risk of meaning-critical omissions, 
    we extract \emph{core events} from each source segment as a minimal semantic representation.
    Concretely, we identify the main predicate and collect its content-bearing arguments, including nouns, proper nouns, and numerals by using using Stanza Chinese POS tagging.\footnote{\url{https://stanfordnlp.github.io/stanza/}}.
    We then measure semantic consistency by computing contextual embedding similarity between source and candidate predicate--argument realizations, and flag a violation if no candidate event sufficiently matches the source core event.
    This predicate--argument abstraction serves as the reference for measuring semantic integrity in compressed translations (via \textit{BT-CERR}).
\end{enumerate}
% \section{The Sand-Glass Benchmark Construction}
% \label{sec:appendix_sand-glass_construction}

% Sand-Glass is designed for \emph{time-constrained} translation, where the output must satisfy a strict temporal budget while preserving the essential meaning.
% Accordingly, the construction emphasizes two components:
% (i) \textbf{duration-aware segmentation} to derive realistic per-segment budgets from speech,
% and (ii) \textbf{core event extraction} to enable a fine-grained semantic retention check under forced compression (used by \textit{BT-CERR} in Section~\ref{sec:evaluation_metrics}).

% \paragraph{Pipeline Overview.}
% Starting from real-world videos, we obtain ASR transcripts, segment them into duration-bounded subtitle units, apply multi-stage quality filtering, and finally extract \emph{core events} (predicate--argument abstractions) for semantic evaluation.

% \paragraph{Construction Procedure.}
% \begin{enumerate}
%     \item \textbf{Subtitle extraction and duration-aware segmentation.}
%     We collect real-world videos and transcribe speech using ASR.
%     The ASR output is then segmented into subtitle units using speech pauses and semantic completeness constraints.
%     Each segment is associated with a temporal budget derived from its speech duration.
%     We additionally remove segments with obvious duration anomalies (e.g., extremely short/long speech spans) to avoid unrealistic budgets.

%     \item \textbf{Subtitle processing and context packaging.}
%     We clean the transcripts by removing background music markers and semantically insignificant utterances (e.g., fillers or non-speech artifacts).
%     To improve contextual coherence for translation and evaluation, we package the data into sliding windows of ten consecutive segments.
%     For standardized model interaction, prompts require outputs in a fixed JSON schema.

%     \item \textbf{Multi-stage quality filtering.}
%     We apply a staged filtering pipeline to ensure that the benchmark is structurally valid, readable, and diverse:
%     \begin{itemize}[nosep,leftmargin=*]
%         \item \textbf{Structural validity.} Remove samples with unparsable formats, inconsistent timestamps (e.g., start time $\ge$ end time), empty/corrupted text, and language--script mismatches.
%         \item \textbf{Duration/statistical sanity.} Discard segments with abnormal durations or extreme characters-per-second (CPS) to ensure basic readability and realistic time constraints.
%         \item \textbf{Lightweight quality signals and de-duplication.} Score remaining samples using inexpensive automatic signals (e.g., repetition/noise ratios and shallow fluency proxies) and filter by a threshold.
%         To avoid over-pruning, we keep borderline cases with reduced sampling weights.
%         We then remove exact and near-duplicates via normalization followed by LSH-based clustering (e.g., LIMIT~\cite{jha2023limit}), keeping only the best instance per cluster.
%         Finally, we perform bucketed quota sampling along key axes (e.g., length, CPS, language, and style) to obtain a balanced yet diverse final corpus.
%     \end{itemize}



\section{Implementation Details}
\label{sec:appendix_hyper}

Our RM training framework is built on Megatron. We use the Qwen3-32B-Chat model as the initialization. The training is conducted with a batch size of 256, using a cosine learning rate scheduler with an initial learning rate of 5e-6. All models are trained on 64  Huawei's Ascend 910B NPUs.

Our RL training framework is based on the Verl framework. We use the Qwen3-8B-Chat model as the initialization for RL training. During training, we configure a batch size of 16 and perform 16 rollouts per prompt using the GRPO algorithm. The learning rate is initialized at 1e-8, and a cosine scheduler with warm-up is applied toward the final iteration. Sampling is conducted with a temperature of 1.0, and the maximum generation length is limited to 1,024 tokens. The KL penalty coefficient $\beta$ is set to 0, effectively removing the KL constraint relative to the reference policy. 
The PPO clipping range $\epsilon$ is fixed at 0.2. All models are trained for one epoch using 8 NVIDIA H800 80G GPUs.
Other detail training hyperparameters are listed in Table \ref{tab:hyperparams}.

Our training set consists of 70K instances drawn from the same data sources as the Sand-Glass benchmark, and is constructed following the same procedure.

\begin{table}[t]
\centering
\small
\setlength{\tabcolsep}{30pt}
\caption{Key hyperparameters used in training HOMURA.}
\begin{tabular}{c c}
\toprule
\textbf{Hyperparameter} & \textbf{Value} \\
\midrule
$\alpha_1 $ & 0.4  \\
$\alpha_2 $ & 0.5  \\
$\lambda_{len} $ & 0.5 \\
$\lambda_{qual} $ & 0.5  \\
$k $ & 300  \\
$\tau_{min} $ & 0  \\
$\tau_{max} $ & 0.8  \\

\bottomrule
\end{tabular}
\label{tab:hyperparams}
\end{table}

\section{Effectiveness of Dynamic Syllable-ratio Reward}
\label{sec:appendix_dynamic_reward}

In Section~\ref{sec:dynamic_reward}, we hypothesized that rigid syllable-ratio bounds are susceptible to discretization noise, particularly in shorter utterances. To validate the necessity of our dynamic relaxation mechanism, we conduct an ablation study comparing our \textit{Dynamic Syllable-ratio Reward} against a static baseline on the Zh$\to$En translation task. Both methods share the same target objective ($\mathcal{B}_L \in [0.8, 0.9]$), but the static version enforces fixed boundaries regardless of source length.

\begin{figure}[h]
    \centering
    \includegraphics[width=\linewidth]{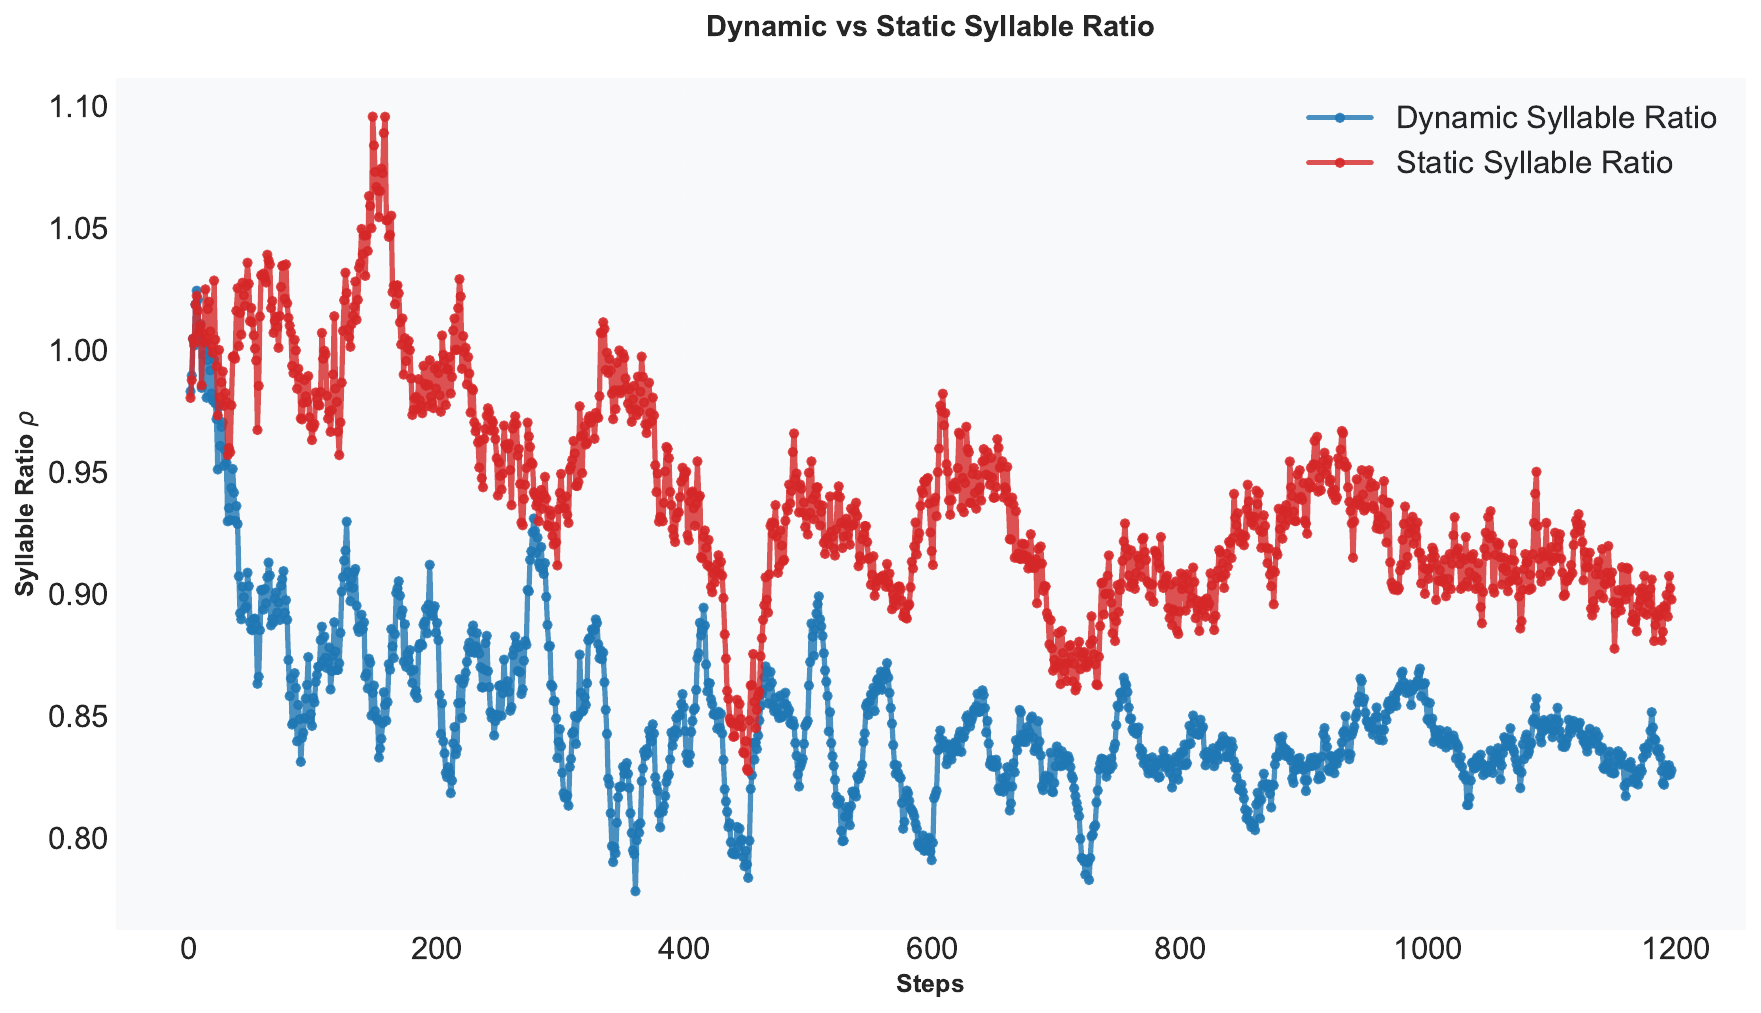}
    \caption{Training dynamics of syllable ratios during policy optimization (Zh$\to$En). The blue curve represents our dynamic bound relaxation, while the red curve represents static fixed bounds. Values indicate the mean syllable ratio $\rho$ across training steps.}
    \label{fig:reward_dynamics}
\end{figure}

As shown in Figure~\ref{fig:reward_dynamics}, the experimental results yield several key observations:

\begin{itemize}
    \item \textbf{Stability and Convergence:} The Dynamic reward (blue) demonstrates significantly smoother optimization and faster convergence into the target interval $[0.8, 0.9]$. In contrast, the Static reward (red) exhibits violent oscillations, especially in early training phases.
    \item \textbf{Mitigating Discretization Noise:} The instability of the static baseline confirms that "hard" rewards for syllable counts are overly sensitive to small variations in short segments. A single-syllable difference in a short sentence can cause a disproportionate jump in the ratio, providing an inconsistent gradient for the RL agent.
    \item \textbf{Optimization Efficiency:} By adaptively relaxing the lower bound for shorter sequences via $\gamma(x)$, our method provides a more continuous and achievable reward landscape. This prevents the model from being penalized for unavoidable linguistic granularity, leading to more efficient learning of the desired compression behavior.
\end{itemize}

These findings justify the use of length-aware dynamic bounds in \textsc{Homura} to ensure stable policy refinement across diverse utterance lengths.

\section{Scaling to Larger Model.}
\label{sec:appendix_scale}

\begin{table}[h]
\centering
\caption{Scaling Analysis of \textsc{Homura} (\text{Zh}$\rightarrow$\text{En}). Comparison between 8B and 32B backbones at $\mathcal{B}_L \in [0.8, 0.9]$.}
\label{tab:scaling_homura}
\footnotesize
\setlength{\tabcolsep}{2.5pt}
\renewcommand{\arraystretch}{1.15}
\begin{tabular}{@{}l l c c c c@{}}
\toprule
\textbf{Scale} & \textbf{Model} & \textbf{IB} & \textbf{Cometkiwi} & \textbf{BT-CERR} & \textbf{BLEU-$\rho$} \\
\midrule
8B 
 & \textbf{HOMURA}\textsubscript{Rubric} & $\checkmark$ & 0.700 & 0.914 & 0.378 \\
 & \textbf{HOMURA}\textsubscript{Reason} & $\checkmark$ & 0.701 & 0.925 & 0.376 \\
\midrule
32B
 & \textbf{HOMURA}\textsubscript{Rubric} & $\checkmark$ & 0.740 & 0.917 & 0.388 \\
 & \textbf{HOMURA}\textsubscript{Reason} & $\checkmark$ &  0.740 & 0.933 & 0.385 \\
\bottomrule
\end{tabular}
\end{table}

We analyze the effect of model scaling by comparing 8B and 32B variants of HOMURA under identical training settings, with results reported in Table \ref{tab:scaling_homura}. Scaling consistently improves translation quality and semantic preservation, as shown by higher BLEU-$\rho$, Cometkiwi and BT-CERR scores. Moreover, the relative advantage of HOMURA\textsubscript{Reason} over HOMURA\textsubscript{Rubric} is preserved at larger scale, suggesting that the proposed reward design scales robustly with model capacity.


\section{Examples of Structured CoT Reasoning for GenRM}
\label{sec_genrm_example_appendix}
This appendix provides illustrative examples of the structured CoT reasoning produced by GenRM.
% \newpage
\begin{tcolorbox}[
  enhanced,
  breakable,
  colback=white,
  colframe=black,
  boxrule=0.6pt,
  left=6pt,right=6pt,top=6pt,bottom=6pt,
  width=\columnwidth
]
\textbf{Structured CoT Example \#1}

\par\smallskip
\textbf{Source sentence (x):}\\
{\small 我曾经在这看到过几艘陌生的船。}

\par\smallskip
\textbf{Translation hypothesis (y):}\\
I have seen a few strange ships here before.

\par\smallskip
\textbf{COT process:}
\begin{enumerate}
  \item \textbf{Back-translation:}
  The translation ``I have seen a few strange ships here before.'' is back-translated into Chinese.
  The back-translation result is {\small ``我以前曾在这里见过几艘奇怪的船。''}
  (I have previously seen several strange ships here).
  Alternatively, it can also be {\small ``我曾经在这里看到过几艘陌生的船。''}
  (I once saw several unfamiliar ships here).

  \item \textbf{Semantic consistency judgment:}
  Compare the source sentence {\small ``我曾经在这看到过几艘陌生的船。''}
  (I once saw several unfamiliar ships here) with the back-translated content
  {\small ``我以前曾在这里见过几艘奇怪的船。''}
  (I have previously seen several strange ships here).
  The two are completely consistent in core semantics, both expressing the fact of
  {\small ``过去在某地看到过不熟悉的船只''} (having seen unfamiliar ships at a certain place in the past).
  {\small ``曾经''} (once / before) corresponds to ``before,''
  {\small ``在这''} (here) corresponds to ``here,''
  {\small ``看到过''} (have seen) corresponds to ``have seen,''
  {\small ``几艘''} (a few) corresponds to ``a few,''
  {\small ``陌生的''} (unfamiliar / strange) corresponds to ``strange,''
  and {\small ``船''} (ships) corresponds to ``ships.''
  The semantic consistency is very high.

  \item \textbf{Translation quality judgment:}
  The translation ``I have seen a few strange ships here before.'' is grammatically correct,
  using the present perfect tense to express a past experience, which conforms to English usage.
  The expression is fluent and natural, with accurate word choice. Therefore, the translation quality is high.
\end{enumerate}

Based on the above, the semantics are consistent and the translation quality is high, resulting in a final score of 1.

\par\smallskip
\textbf{Score:}\\
1
\end{tcolorbox}

\begin{tcolorbox}[
  enhanced,
  breakable,
  colback=white,
  colframe=black,
  boxrule=0.6pt,
  left=6pt,right=6pt,top=6pt,bottom=6pt,
  width=\columnwidth
]
\textbf{Structured CoT Example \#2}

\par\smallskip
\textbf{Source sentence (x):}\\
{\small 所以天命人只有超度了金池长老的冤魂}

\par\smallskip
\textbf{Translation hypothesis (y):}\\
So the Mandate Person can only rescue the lingering soul of Jinchi Elder

\par\smallskip
\textbf{COT process:}
\begin{enumerate}
  \item \textbf{Back-translation:}
  The translation ``So the Mandate Person can only rescue the lingering soul of Jinchi Elder''
  is back-translated into Chinese as
  {\small ``所以天命人只能解救金池长老逗留的灵魂。''}
  (So the Mandate Person can only rescue the lingering soul of Elder Jinchi).

  \item \textbf{Semantic consistency judgment:}
  The key terms in the source text are {\small ``超度''} (perform salvation rites / help a soul attain deliverance)
  and {\small ``冤魂''} (wronged or vengeful spirit).
  {\small ``超度''} is a term with strong religious and cultural connotations, referring to helping the deceased soul
  attain liberation and enter reincarnation or the afterlife through rituals.
  However, the word ``rescue'' in the translation is overly general and fails to convey the deeper religious meaning
  of {\small ``超度''}.
  {\small ``冤魂''} refers to a ghost that died unjustly and carries strong resentment, whereas ``lingering soul''
  {\small (逗留的灵魂)} only expresses the idea of lingering or wandering, losing the core semantic component of
  {\small ``冤''} (wronged / resentful).
  Therefore, the back-translated content is semantically inconsistent with the original text.

  \item \textbf{Translation quality judgment:}
  Due to the semantic inconsistency, this step is skipped.
\end{enumerate}

Based on the above analysis, the semantics are inconsistent, and the final score is 0.

\par\smallskip
\textbf{Score:}\\
0
\end{tcolorbox}

\section{Prompt for Linguistic well-formedness Reward.}
\label{sec:prompt_fluency}

This appendix provides the training prompt used for the linguistic well-formedness reward.

\begin{tcolorbox}[
  enhanced,
  colback=white,
  colframe=black,
  boxrule=0.6pt,
  left=6pt,right=6pt,top=6pt,bottom=6pt,
  width=\columnwidth,
  breakable
]
\textbf{Training Prompt}

You are an expert in \{target\_lang\} translation.
Given context \texttt{<context>} for background reference.
Here is a text \texttt{<text>} from the context and its corresponding
\{target\_lang\} translation \texttt{<translation>}.
You need to determine whether \texttt{<translation>} is a qualified
\{target\_lang\} translation.

\medskip
\textbf{Requirements:} Consider only the following criteria; if any are
not met, the score is 0:
\begin{enumerate}
  \item \textbf{Grammaticality:}
  No obvious grammatical or syntactic errors, consistency errors
  (e.g., subject--verb agreement, tense, case, gender/number),
  collocation errors, or linguistic defects caused by punctuation or spelling.
  \item \textbf{Readability \& Coherence:}
  The sentence structure is complete, logically coherent, and naturally
  connected, making it smooth and easy to understand; there should be no
  obvious fragmentation, garbled text, repetitive stacking, or malformed
  sentences.
\end{enumerate}

\medskip
\textbf{Input:}

\texttt{<context>}: \{context\}

\texttt{<text>}: \{text\}

\texttt{<translation>}: \{translation\}

\medskip
\textbf{Output Requirements:}
\begin{itemize}
  \item If \texttt{<translation>} satisfies both criteria above, return
  \texttt{<<1>>}.
  \item Otherwise, return \texttt{<<0>>}.
  \item Please output \texttt{<<0>>} or \texttt{<<1>>} directly; do not
  output any explanation.
\end{itemize}

\textbf{Output:}
\end{tcolorbox}

\section{Ablation of GenRM Design}
\label{sec_genrm_compare_appendix}
This appendix presents an ablation study on the design of the reward model within the GenRM framework. In particular, we compare our self-trained GenRM with an external LLM-as-RM. In this ablation, the external reward model fully replaces GenRM, while all other components of the compression-oriented reinforcement learning pipeline are kept identical.

\paragraph{External LLM-as-RM Setup} For the external reward model baseline, we adopt an LLM-as-RM setup using \texttt{DeepSeek-V3}. Given a source sentence and its translation, the model is prompted to perform a quality assessment. Specifically, it evaluates whether the translation (i) preserves the core semantic content of the source sentence under the target syllable constraint, and (ii) remains fluent and grammatical. The model outputs a binary acceptability judgment, which is directly used as the reward signal during policy optimization.
The prompt for external LLM-as-RM is below:

\begin{tcolorbox}[
  enhanced,
  breakable,
  colback=white,
  colframe=black,
  boxrule=0.6pt,
  left=6pt,right=6pt,top=6pt,bottom=6pt,
  width=\columnwidth
]
\textbf{Prompt for GenRM}

\vspace{0.5em}

You are a translation quality reward model (GenRM).

Given contextual information, a source sentence, and its translation, you will perform step-by-step reasoning to assess translation quality. Your evaluation process must strictly follow the sequence below.

\textbf{Step 1: Back-Translation} \\
Translate the given translation back into the source language.

\textbf{Step 2: Semantic Consistency Assessment} \\
Compare the semantic consistency between the original source text and the back-translated text.
\begin{itemize}
  \item If the meanings are consistent or highly consistent, proceed to Step~3.
  \item If they are inconsistent, skip Step~3 and assign a final score of~0.
\end{itemize}

\textbf{Step 3: Translation Quality Assessment} \\
Evaluate whether the translation is of high quality based on factors such as fluency, grammatical correctness, and cultural appropriateness.

\vspace{0.5em}

Your final output must include a clear chain-of-thought reasoning process and a reward score:
\begin{itemize}
  \item If semantic consistency is satisfied and the translation quality is high,
        set \texttt{score = 1}.
  \item Otherwise, set \texttt{score = 0}.
\end{itemize}

\vspace{0.5em}

\textbf{Output Format} \\
The output must strictly follow the format below. Do not add or omit any fields:
\begin{quote}\ttfamily
\noindent
\{\\
"COT": "<COT reasoning>", \\
"score": 0 or 1 \\
\}
\end{quote}

\textbf{Input Format} \\
Context: \texttt{\{context\}} \\
Source text: \texttt{\{current\_text\}} \\
Translation: \texttt{\{translated\_text\}}
\end{tcolorbox}



\paragraph{Results and Analysis} Table~\ref{tab:ablation_study} compares compression translation models optimized with different reward model designs. The model trained with the self-trained GenRM consistently outperforms its counterpart using an external LLM-as-RM baseline, demonstrating that a reward model trained specifically for compression-oriented translation provides more effective optimization guidance than a generic, prompt-based evaluator.

\begin{table}[ht]
    \centering
    \caption{Effect of GenRM choice on compressed translation under HOMURA\textsubscript{Reason} (Average across all language pairs).}
    \label{tab:ablation_study}

    \footnotesize
    \setlength{\tabcolsep}{1pt}
    \renewcommand{\arraystretch}{0.95}

    \resizebox{0.6\linewidth}{!}{%
    \begin{tabular}{lccc}
        \toprule
        \textbf{Model Variant} & \textbf{Cometkiwi} & \textbf{BT-CERR} & \textbf{BLEU-$\rho$} \\
        \midrule
        HOMURA\textsubscript{Reason}  & 0.636 & 0.881 & 0.335 \\
        \midrule
        HOMURA\textsubscript{Reason} (w/ External RM)  &  0.628& 0.879 & 0.330 \\
        \bottomrule
    \end{tabular}%
    }
\end{table} 


\section{Case Study}
\label{sec:appendix_cases}

This appendix provides a fine-grained analysis of the linguistic strategies employed by \textsc{Homura} to navigate the quality-compression frontier. Unlike standard LLMs that often rely on simple truncation, our model learns a hierarchy of compression operations.

\paragraph{Observation 1: Taxonomic Shifts in Semantic Packing.} 
Analysis of Table~\ref{tab:combined_case_study} reveals three distinct tiers of semantic packing performed by \textsc{Homura} as constraints tighten:
\begin{itemize}[nosep]
    \item \textbf{Lexical Consolidation}: Mapping verbose multi-word phrases to high-density synonyms (e.g., the 7-syllable ``relationship between them'' $\rightarrow$ 1-syllable ``bond'').
    \item \textbf{Aspectual Simplification}: Reducing periphrastic verbal constructions into synthetic forms (e.g., ``is becoming closer'' $\rightarrow$ ``grows closer''), which preserves the temporal aspect while reducing syllable count.
    \item \textbf{Syntactic Pruning}: Selectively removing low-surprisal functional tokens (articles, auxiliaries) while anchoring the sentence around core predicate-argument structures.
\end{itemize}

\paragraph{Observation 2: Behavioral Transition at the Compression Wall.} 
The trade-off spectrum in Part 2 of Table~\ref{tab:combined_case_study} visualizes the transition from naturalistic translation to ``telegraphic speech.'' While fluency is maintained down to $\rho \approx 0.50$, pushing toward the empirical limit ($\rho \approx 0.25$) forces the model to prioritize \textit{propositional content} over \textit{morphosyntactic correctness}. This behavior confirms that HOMURA does not randomly drop tokens but strategically re-allocates the syllable budget to the most informative constituents (e.g., ``Bond grows tighter''), ensuring minimal meaning loss even at the threshold of reward collapse.

\begin{table*}[!ht]
    \centering
    \caption{Qualitative Case Study on $\text{Zh}\rightarrow\text{En}$: Comparison between frontier LLMs and \textsc{Homura} across varying compression intensities. Source: \textbf{两人之间的关系越来越亲密} (12 syllables).}
    \label{tab:combined_case_study}
    \footnotesize
    \setlength{\tabcolsep}{5pt}
    \renewcommand{\arraystretch}{1.2}
    \begin{tabularx}{\linewidth}{l l X c c p{0.25\textwidth}}
        \toprule
        \textbf{Category} & \textbf{Model} & \textbf{Output Text} & \textbf{Syl.} & $\boldsymbol{\rho}$ & \textbf{Quality Observation} \\
        \midrule
        \multicolumn{6}{l}{\textit{Part 1: Comparison with Baselines (Target $\rho \in [0.8, 0.9]$ for Prompted Models)}} \\
        \multirow{3}{*}{Unconstrained} 
            & Claude-4.1-Opus & The relationship between the two is becoming increasingly intimate. & 20 & 1.67 & Naturally verbose; high fidelity. \\
            & Gemini-2.5-Pro  & The relationship between the two grew increasingly intimate. & 17 & 1.42 & Fluent but ignores brevity. \\
            & GPT-5           & The relationship between the two is growing increasingly close. & 17 & 1.42 & Optimal quality; no length control. \\
        \cmidrule(lr){1-6}
        \multirow{3}{*}{\shortstack[l]{Prompt-based\\Compression}}  
            & Claude-4.1-Opus & Their relationship grows increasingly intimate. & 13 & 1.08 & Fails to reach target interval. \\
            & Gemini-2.5-Pro  & Their relationship is growing more intimate. & 12 & 1.00 & Fails to reach target interval. \\
            & GPT-5           & The two are becoming more and more intimate. & 12 & 1.00 & Fails to reach target interval. \\
        \midrule
        \multicolumn{6}{l}{\textit{Part 2: Controllable Compression via \textsc{Homura} ($\rho$ Trade-off Analysis)}} \\
        \textsc{Homura} & $\rho \approx 1.25$ & The relationship between the two is becoming closer. & 15 & 1.25 & Full fidelity and naturalness. \\
        & $\rho \approx 0.83$ & The bond between them is growing closer. & 10 & 0.83 & \textbf{Precise adherence} via condensation. \\
        & $\rho \approx 0.58$ & Bond between them grows closer. & 7 & 0.58 & Minor grammatical omission. \\
        & $\rho \approx 0.50$ & Their bond grows closer. & 6 & 0.50 & Extreme brevity; core meaning only. \\
        & $\rho \approx 0.25$ & Bond grows tighter. & 3 & 0.25 & \textbf{Compression Limit}; loss of fluency. \\
        \bottomrule
    \end{tabularx}
\end{table*}


\section{Detailed Breakdown of Expansion Metrics}
\label{sec:appendix_noraml_roundtrip_metrics}

\begin{figure*}[t]
\centering
\includegraphics[width=0.95\textwidth]{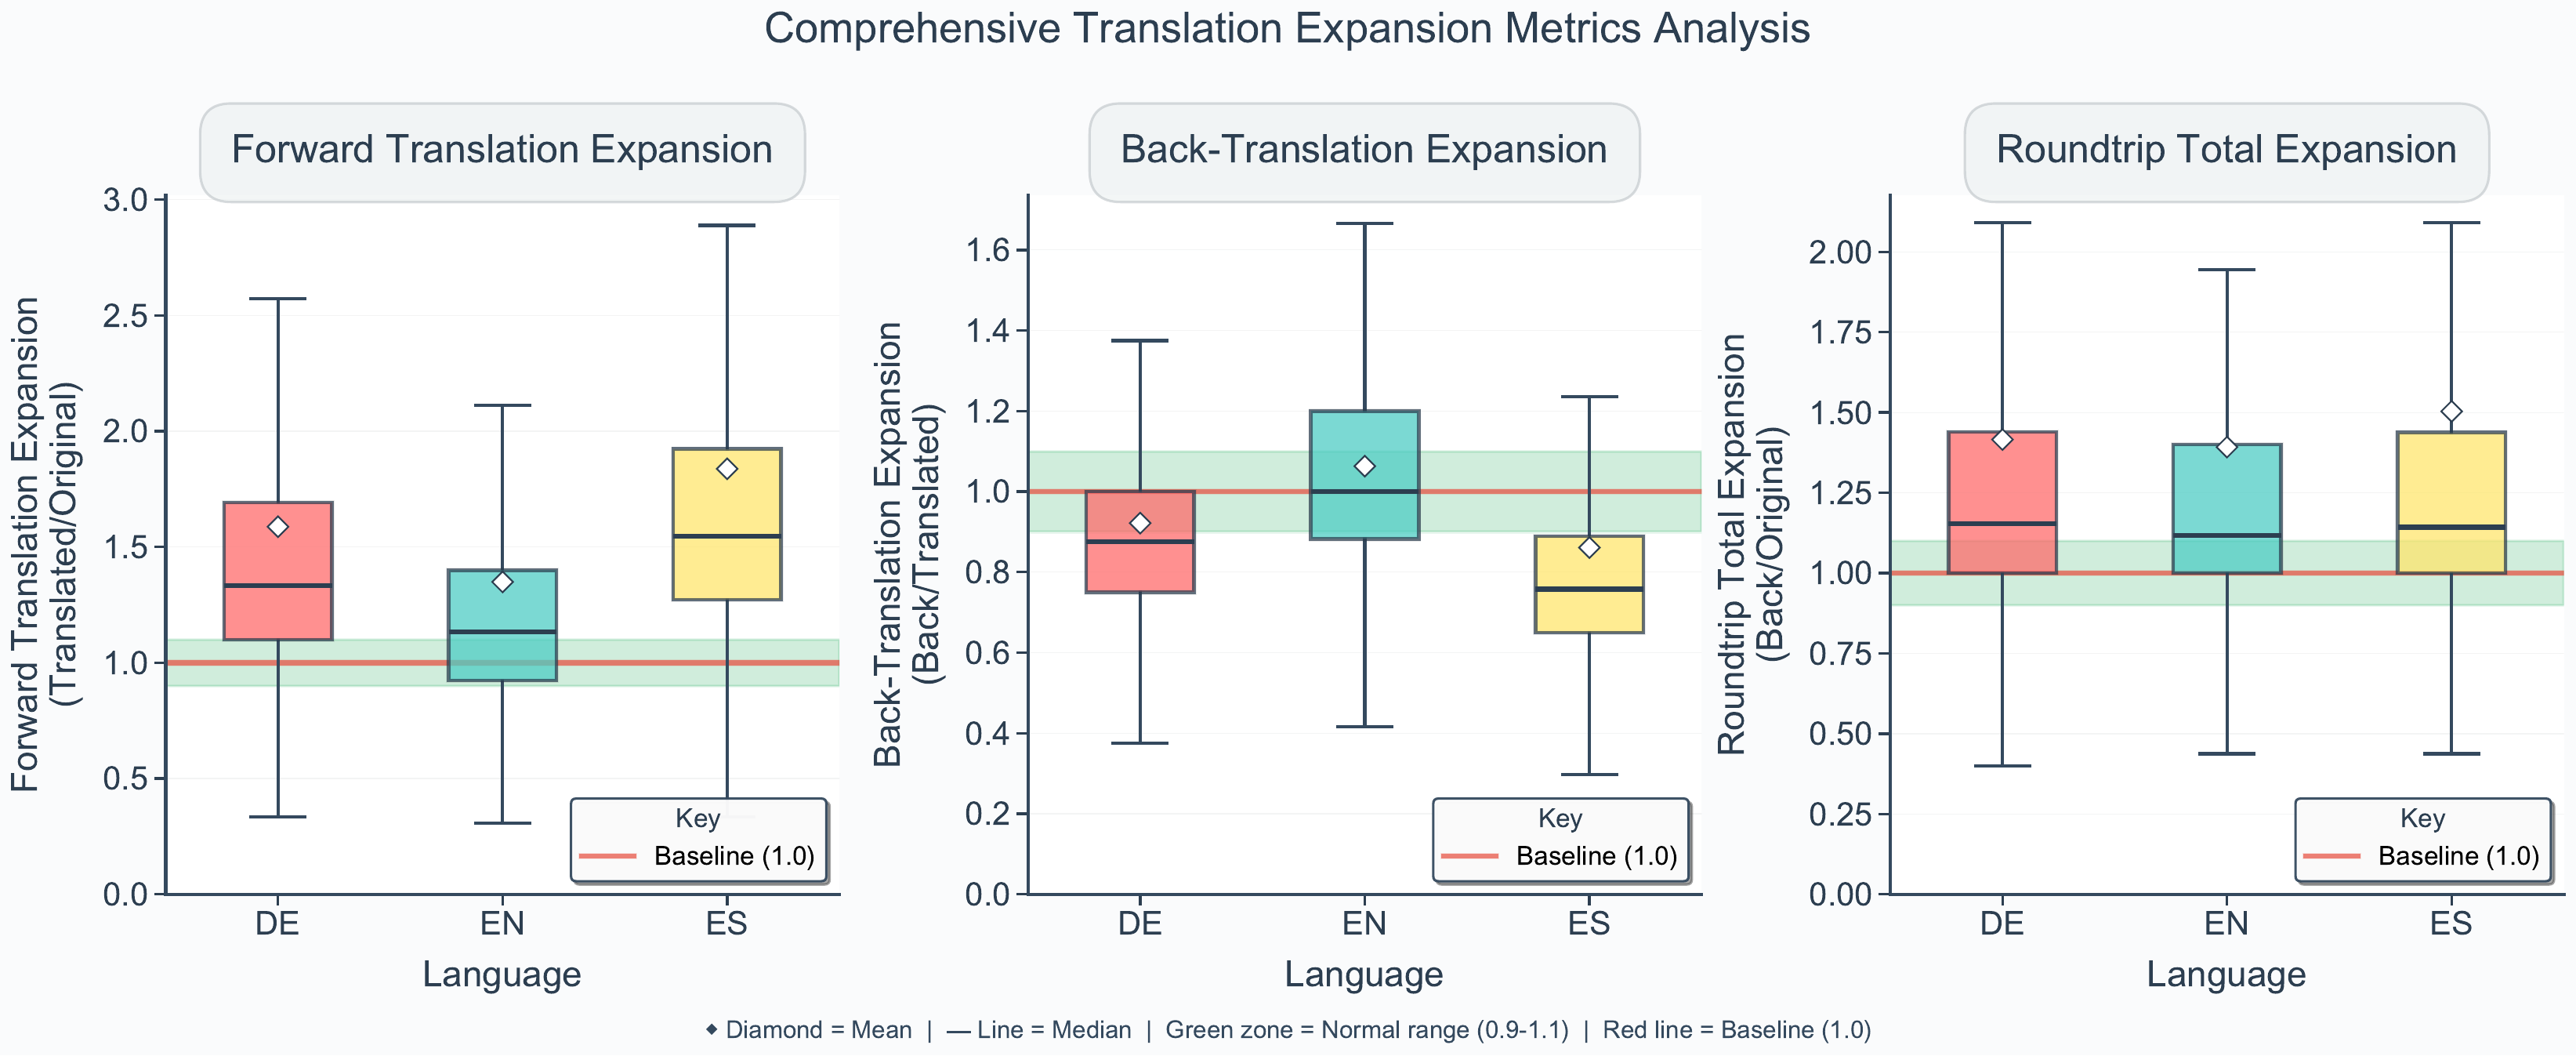}
\vspace{-2mm}
\caption{Statistical distribution of translation expansion metrics across DE, EN, and ES. The boxplots illustrate the variations in Forward, Back, and Roundtrip expansion ratios, with diamonds indicating means.}
\label{fig:boxplot_three_metrics}
\vspace{-3mm}
\end{figure*}

To provide a comprehensive view of the verbosity bias identified in Section~\ref{sec:pilot}, we present a fine-grained statistical breakdown of expansion metrics across various frontier LLMs and language pairs. As summarized in Table~\ref{tab:detailed_metrics}, the \textit{Roundtrip Expansion Ratio} ($R_{rtp}$) consistently exceeds the unity baseline across all tested models and languages, with a high percentage of segments ($>60\%$) exhibiting systemic inflation. 

The distribution shifts visualized in Figure~\ref{fig:boxplot_three_metrics} further confirm that this bias is not merely a result of specific difficult cases but represents a structural characteristic of current LLM-based translation. 

%\FloatBarrier
\begin{table*}[!th]
\centering
\caption{Detailed Breakdown of Expansion Metrics across Models and Language Pairs. $R_{fwd}$, $R_{bwd}$, and $R_{rtp}$ denote Forward, Backward (Back-translation), and Roundtrip Expansion Ratios, respectively. Values are presented as Mean and Standard Deviation.}
\label{tab:detailed_metrics}
\small
% 使用 tabular* 强制铺满页面宽度，@{\extracolsep{\fill}} 会自动撑开列间距
\begin{tabular*}{\textwidth}{@{\extracolsep{\fill}}llcccc@{}}
\toprule
\textbf{Language} & \textbf{Model} & \textbf{$R_{fwd}$ (Mean $\pm$ Std)} & \textbf{$R_{bwd}$ (Mean $\pm$ Std)} & \textbf{$R_{rtp}$ (Mean $\pm$ Std)} & \textbf{$R_{rtp} > 1$ (\%)} \\ \midrule

\multirow{5}{*}{\textbf{De}} 
 & \texttt{claude-4.1-opus} & $1.58 \pm 0.96$ & $0.95 \pm 1.54$ & $1.39 \pm 0.99$ & 66.2 \\
 & \texttt{deepseek-v3} & $1.67 \pm 1.37$ & $0.91 \pm 0.29$ & $1.54 \pm 1.89$ & 63.8 \\
 & \texttt{gemini-2.5-pro} & $1.51 \pm 0.88$ & $0.96 \pm 0.44$ & $1.35 \pm 0.84$ & 59.0 \\
 & \texttt{gpt-5} & $1.63 \pm 0.96$ & $0.90 \pm 0.19$ & $1.43 \pm 0.87$ & 71.8 \\ \midrule

\multirow{5}{*}{\textbf{En}} 
 & \texttt{claude-4.1-opus} & $1.36 \pm 1.13$ & $1.07 \pm 0.55$ & $1.41 \pm 1.32$ & 64.8 \\
 & \texttt{deepseek-v3} & $1.41 \pm 1.15$ & $1.05 \pm 0.48$ & $1.47 \pm 1.71$ & 59.1 \\
 & \texttt{gemini-2.5-pro} & $1.29 \pm 0.81$ & $1.07 \pm 0.25$ & $1.33 \pm 0.80$ & 61.0 \\
 & \texttt{gpt-5} & $1.33 \pm 0.81$ & $1.07 \pm 0.23$ & $1.36 \pm 0.80$ & 65.9 \\ \midrule

\multirow{5}{*}{\textbf{Es}} 
 & \texttt{claude-4.1-opus} & $1.81 \pm 1.05$ & $0.90 \pm 2.48$ & $1.41 \pm 1.19$ & 66.9 \\
 & \texttt{deepseek-v3} & $1.99 \pm 1.83$ & $1.01 \pm 1.12$ & $1.99 \pm 2.90$ & 64.0 \\
 & \texttt{gemini-2.5-pro} & $1.72 \pm 0.99$ & $0.83 \pm 0.36$ & $1.35 \pm 0.87$ & 60.4 \\
 & \texttt{gpt-5} & $1.86 \pm 1.09$ & $0.78 \pm 0.18$ & $1.40 \pm 0.83$ & 68.5 \\ \bottomrule
\end{tabular*}
\end{table*}
%\FloatBarrier

\newpage

\section{Analysis of Regularization Strength}
\label{app:stability_analysis}

In Eq.\eqref{eq:kl-regularized-rl}, $\beta$ controls the trade-off between control strength and adherence to the reference model $P_0$. Our experiments show that $\beta \to 0$ leads to better syllable-ratio compliance and linguistic quality. This appendix justifies how HOMURA maintains training stability and semantic integrity even without explicit KL regularization ($\beta=0$).

\section*{M.1 Theoretical Justification: Stability through Implicit Regularization}

A common concern in RLHF is that removing the token-level KL penalty ($\beta=0$) may lead to training instability. However, we argue that for time-constrained translation, the explicit KL penalty defined in Eq. (\ref{eq:kl-regularized-rl}) is not only detrimental but also redundant, as its stabilizing role is effectively superseded by the internal dynamics of our framework.

\paragraph{Escaping the Verbosity Trap.} 
Standard RLHF uses token-level KL divergence to anchor the policy to a pre-trained reference $P_0$. In the Sand-Glass task, the model must perform significant structural compression to meet strict temporal constraints. A rigid KL penalty treats these necessary structural deviations as distributional shifts, mathematically penalizing the model for being concise and confining it to the verbose distribution of the base model. By setting $\beta = 0$, we transition from \textit{distribution matching} to \textit{goal-oriented optimization}, allowing the model to prioritize control strength and efficiency.

\paragraph{Sufficiency of Implicit Regularization.} 
The stability typically provided by the KL term is maintained through two alternative forces:

\begin{itemize}[leftmargin=1.5em]
    \item \textbf{Token-level Trust Region (GRPO Dynamics):} 
    Numerical stability is preserved via the surrogate loss function $\mathcal{L}_{GRPO}$, which integrates two complementary token-level stabilizing forces:
    \begin{equation}
        \mathcal{L}_{GRPO}(\theta) = \frac{1}{G} \sum_{i=1}^{G} \sum_{t=1}^{T} \min \left( r_{i,t}(\theta) \hat{A}_i, \text{clip}(r_{i,t}(\theta), 1-\epsilon, 1+\epsilon) \hat{A}_i \right)
    \end{equation}
    where the advantage $\hat{A}_i$ is normalized within the group: $\hat{A}_i = (R_i - \mu_{\text{group}})/\varsigma_{\text{group}}$. 
    
    The \textit{clipping mechanism} enforces a trust region relative to the evolving policy $\pi_{\theta_{old}}$, preventing abrupt updates. Simultaneously, the \textit{group-relative normalization} centers updates around the group's moving average. This relative anchoring ensures the policy explores the length-constrained space without global drift.

    \item \textbf{Sequence-level Implicit Semantic Regularization ($R_{bt}$):} 
    While the token-level KL constraint is removed, the policy is still constrained at the sequence level by the structural-agnostic back-translation reward $R_{bt}$. This acts as an \textit{implicit semantic regularizer}: it does not penalize \textit{how} the model expresses information (lexical choice), but rather \textit{whether} the information is preserved (semantic fidelity). This sequence-level anchoring allows the model to explore radical syntactic restructuring for conciseness while ensuring the output remains a faithful translation.
\end{itemize}

In summary, the synergy between GRPO's token-level trust region and the sequence-level semantic anchor of $R_{bt}$ provides a sufficient regularizing effect. This allows \textit{HOMURA} to escape the reference's verbosity trap and navigate the complex rate-distortion frontier required for high-precision synchronization.


\subsection{Empirical Analysis}

We analyze the training dynamics across different KL coefficients $\beta \in \{0, 0.01, 0.05\}$ in Figure \ref{fig:five_panel_dynamics}.

\begin{figure*}[htbp]
    \centering
    \includegraphics[width=\textwidth]{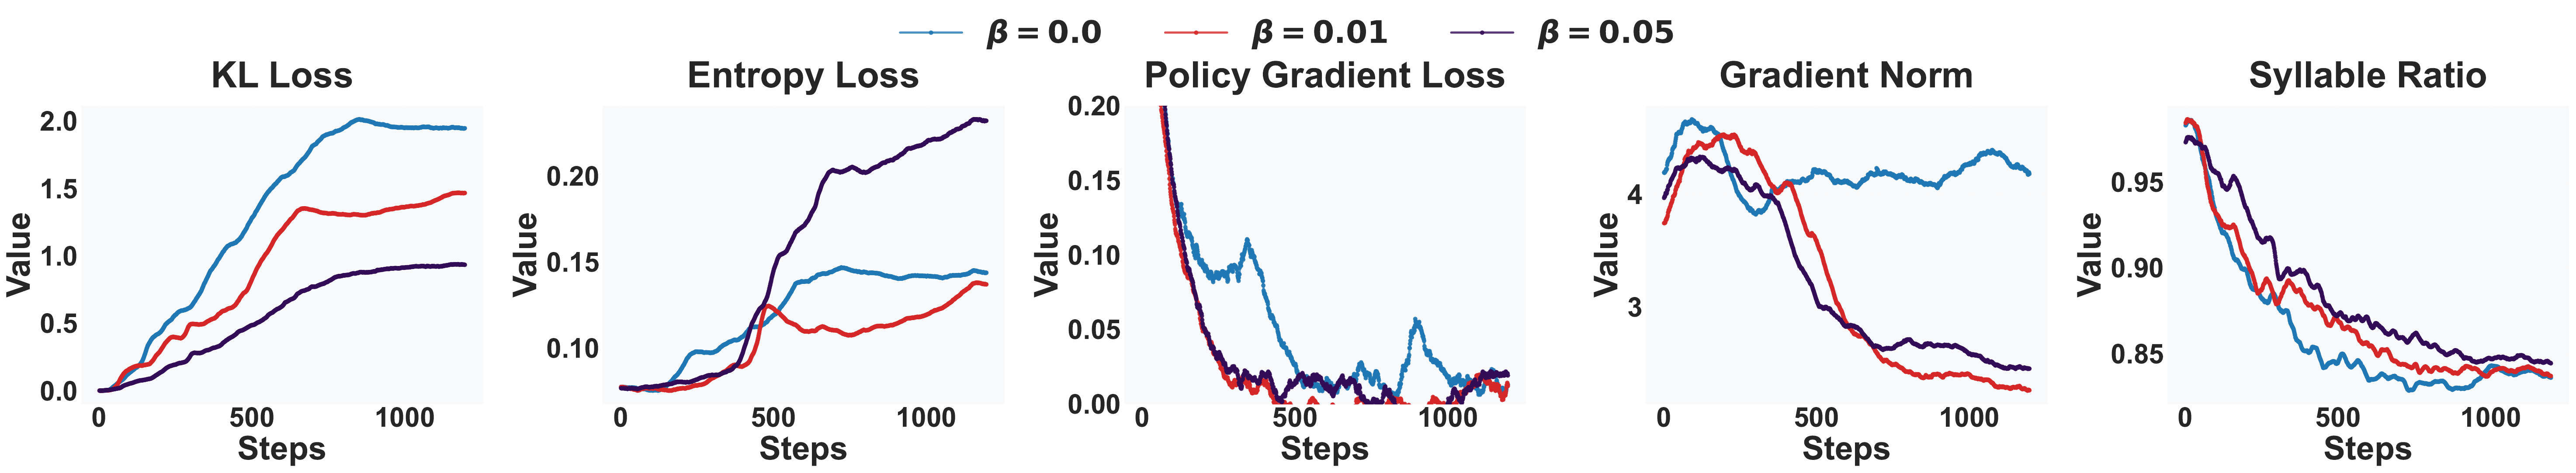}
    \caption{Training dynamics for varying $\beta$. The $\beta=0$ variant (light blue) maintains a stable gradient norm and policy entropy, indicating effective exploration without optimization stagnation.}
    \label{fig:five_panel_dynamics}
\end{figure*}

\paragraph{Training Dynamics and Gradient Norms.}
As shown in Figure \ref{fig:five_panel_dynamics}, the $\beta=0$ regime (light blue) demonstrates superior optimization vitality. Without the KL constraint, the model maintains a stable Gradient Norm ($\sim$4.0) and a healthy Policy Gradient Loss. In contrast, the $\beta=0.05$ variant (purple) shows a significant increase in policy entropy mid-training followed by a stagnating gradient norm. This suggests that a high KL penalty creates conflicting objectives between length compliance and reference faithfulness, leading to inefficient policy updates where the model fails to find a clear optimization direction.

\paragraph{Performance Trade-offs: The Pruning vs. Rewriting.}
Table \ref{tab:beta_comparison} shows the impact of $\beta$ on final metrics. While all configurations achieve the target syllable budget, their linguistic strategies differ significantly:

\begin{table}[h]
\centering
\caption{Impact of $\beta$ on performance. $\beta=0$ achieves the best balance between compression and fidelity, as indicated by BT-CERR and BLEU-$\rho$.}
\label{tab:beta_comparison}
\begin{tabular}{lcccc}
\toprule
Configuration & IB & COMET  & BT-CERR  & BLEU-$\rho$  \\ \midrule
$\beta = 0$  & $\checkmark$ & 0.700          & \textbf{0.914} & \textbf{0.378}     \\
$\beta = 0.01$ & $\checkmark$     & 0.708 & 0.874          & 0.332             \\
$\beta = 0.05$  & $\checkmark$     & 0.711 & 0.879          & 0.359               \\ \bottomrule
\end{tabular}
\end{table}

The $\beta = 0$ configuration yields the highest BT-CERR and BLEU-$\rho$, outperforming all regularized settings. This indicates that removing the token-level prior is essential for structural adaptation—the model's ability to fundamentally rewrite sentences for conciseness rather than just deleting words. Higher $\beta$ values force the model into a conservative strategy: it adheres closely to the reference's lexical surface to satisfy the KL penalty (maintaining higher COMET), but fails to achieve optimal structural efficiency (lower BT-CERR), which is critical for high-precision synchronization in time-constrained scenarios.



\section{Declaration of AI Assistance}
To enhance development efficiency, GitHub Copilot was utilized as a coding assistant in this study. Specifically, it facilitated the implementation of data preprocessing modules, the execution of statistical analyses, and the rendering of complex experimental figures. The core algorithmic design, reinforcement learning frameworks, and the interpretation of results remain the original work of the authors, who maintain full responsibility for the code's accuracy.

% In the preparation of this work, we used Gemini to improve the readability and language quality of the manuscript. The authors assume full responsibility for the content, including the verification of AI-generated text and visual elements.
